# Supplementary material for: A Volume-based Description of Transport in Incompressible Liquid Electrolytes and its Application to Ionic Liquids
Source: arXiv:2209.05769 ancillary file (2023-10-20)
Supplement: Supplementary file 1 [file SupplementaryInformation.pdf]

# Supporting Information: A Volume-based Description of Ion Transport: The Role of Incompressibility

Franziska Kilchert,[†,‡] Martin Lorenz,[¶] Max Schammer,[†,‡] Pinchas Nürnberg,[¶] Monika Schönhoff,[¶] Arnulf Latz,[†,‡,§] and Birger Horstmann[*,†,‡,§]

†*German Aerospace Center, Pfaffenwaldring 38-40, 70569 Stuttgart, Germany*

‡*Helmholtz Institute Ulm, Helmholtzstraße 11, 89081 Ulm, Germany*

¶*University of Münster, Corrensstraße 28/30, 48149 Münster, Germany*

§*Universität Ulm, Albert-Einstein-Allee 47, 89081 Ulm, Germany*

E-mail: birger.horstmann@dlr.de

# Contents

**S-1 Theory** **S-2**

S-1.1 Convection Equation . . . . . . . . . . . . . . . . . . . . . . . . . . . . . . S-2

S-1.2 Reduced Description (Mass-based Frame) . . . . . . . . . . . . . . . . . . . . . S-3

S-1.3 Transformation of Transference Numbers . . . . . . . . . . . . . . . . . . . . . S-4

**S-2 Experimental Validation** **S-4**

S-2.1 Binary Systems . . . . . . . . . . . . . . . . . . . . . . . . . . . . . . . . . S-4

S-2.2 Ternary Systems . . . . . . . . . . . . . . . . . . . . . . . . . . . . . . . . . S-4

**References** **S-7**

# S-1 Theory

## S-1.1 Convection Equation

In Ref. S1, we derived an equation for the convection velocity $\mathbf{v}^{\mathrm{m}}$. This derivation was based on the extensivity of the volume and on the Euler equations for the volume.

Here, we show that our derivation can be applied to different choices for the drift velocity as well. To see this, we consider the variation of the Euler equation for the volume (see eq. (4)), $0 = \sum_{\alpha=1}^{\mathrm{N}} \delta(c_\alpha \nu_\alpha) = \sum_{\alpha=1}^{\mathrm{N}}(\delta c_\alpha \cdot \nu_\alpha + c_\alpha \cdot \delta\nu_\alpha)$. In Ref. S1 we showed that this variation of the Euler equation reduces to concentration variations alone,

$$0 = \sum_{\alpha=1}^{\mathrm{N}} \nu_\alpha \cdot \delta c_\alpha, \tag{S-1}$$

Note that the result eq. (S-1) is frame-invariant. However, it can be evaluated with respect to any reference frame via taking the time evolution for the variation $\delta c_\alpha \rightarrow \mathrm{D}^\psi c_\alpha/\mathrm{d}t = -c_\alpha \nabla \mathbf{v}^\psi - \nabla \mathcal{N}_\alpha^\psi$. Here, the frame-dependent derivative operator is defined by $\mathrm{D}^\psi/\mathrm{d}t = \partial/\partial t + \mathbf{v}^\psi \cdot \nabla$,[S2] and formalizes

the transport equation for the species concentrations. Thus, in the mass description, we find

$$\nabla \mathbf{v}^{\mathrm{m}} = -\sum_{\alpha=1}^{\mathrm{N}} \nu_\alpha \cdot \nabla \mathcal{N}_\alpha^{\mathrm{m}}, \tag{S-2}$$

and in the reduced form

$$\nabla \mathbf{v}^{\mathrm{m}} = -\frac{\tilde{\nu}_2^{\mathrm{m}}}{F \tilde{z}_2^{\mathrm{m}}} \nabla \mathcal{J}^{\mathrm{m}} - \sum_{\alpha=3}^{\mathrm{N}} \tilde{\tilde{\nu}}_\alpha^{\mathrm{m}} \cdot \nabla \mathcal{N}_\alpha^{\mathrm{m}}, \tag{S-3}$$

with

$$\tilde{z}_\alpha^{\mathrm{m}} = z_\alpha - z_1 \cdot M_\alpha / M_1, \quad \tilde{\nu}_\alpha^{\mathrm{m}} = \nu_\alpha - \nu_1 \cdot M_\alpha / M_1, \quad \text{and} \quad \tilde{\tilde{\nu}}_\alpha^{\mathrm{m}} = \tilde{\nu}_\alpha^{\mathrm{m}} - \tilde{\nu}_2^{\mathrm{m}} \cdot \tilde{z}_\alpha^{\mathrm{m}} / \tilde{z}_2^{\mathrm{m}}. \tag{S-4}$$

Whereas in the volume description, we find

$$\nabla \mathbf{v}^{\mathrm{v}} = -\sum_{\alpha=1}^{\mathrm{N}} \nu_\alpha \cdot \nabla \mathcal{N}_\alpha^{\mathrm{v}}, \tag{S-5}$$

and in the reduced form

$$\nabla \mathbf{v}^{\mathrm{v}} = -\frac{1}{F}\left(\nu_2 \nabla \frac{\mathcal{J}^{\mathrm{v}}}{\tilde{z}_2^{\mathrm{v}}} - \nu_1 \nabla \frac{\nu_2}{\nu_1} \frac{\mathcal{J}^{\mathrm{v}}}{\tilde{z}_2^{\mathrm{v}}}\right) + \sum_{\alpha=3}^{\mathrm{N}} \left(\nu_2 \nabla \frac{\tilde{z}_\alpha^{\mathrm{v}}}{\tilde{z}_2^{\mathrm{v}}} \mathcal{N}_\alpha^{\mathrm{v}} - \nu_1 \nabla \frac{\nu_2}{\nu_1} \frac{\tilde{z}_\alpha^{\mathrm{v}}}{\tilde{z}_2^{\mathrm{v}}} \mathcal{N}_\alpha^{\mathrm{v}} - \nu_\alpha \nabla \mathcal{N}_\alpha^{\mathrm{v}} + \nu_1 \nabla \frac{\nu_\alpha}{\nu_1} \mathcal{N}_\alpha^{\mathrm{v}}\right), \tag{S-6}$$

with

$$\tilde{z}_\alpha^{\mathrm{v}} = z_\alpha - z_1 \cdot \nu_\alpha / \nu_1. \tag{S-7}$$

### S-1.2 Reduced Description (Mass-based Frame)

Via mass and charge conservation the number of independent species is reduced by two. From the Euler equation for the volume, eq. (4), follows directly for $c_1$

$$c_1 = \frac{1}{\nu_1}\left(1 - \nu_2 c_2 - \sum_{\alpha=3}^{\mathrm{N}} \nu_\alpha c_\alpha\right). \tag{S-8}$$

Using this expression together with charge conservation, $\varrho = F\sum_{\alpha=1}^{\mathrm{N}} z_\alpha c_\alpha$, we can determine $c_2$

$$c_2 = \frac{z_1 - \nu_1\varrho/F}{\nu_2 z_1 - \nu_1 z_2} + \sum_{\alpha=3}^{\mathrm{N}} c_\alpha \frac{\nu_\alpha z_1 - \nu_1 z_\alpha}{\nu_1 z_2 - \nu_2 z_1}, \tag{S-9}$$

where $\varrho$ is the charge density. Thus, in the electroneutral case ($\varrho = 0$) the first term vanishes.

### S-1.3 Transformation of Transference Numbers

The transformation rule for the transference numbers, eq. (35), can be directly obtained from the frame transformation of the fluxes, eq. (25), by inserting the relations between fluxes and transference numbers,

$$\mathcal{N}_\alpha^{\mathrm{v}} = t_\alpha^{\mathrm{v}}/Fz_\alpha \cdot \mathcal{J}, \tag{S-10}$$

and

$$\mathcal{N}_\alpha^{\mathrm{m}} = t_\alpha^{\mathrm{m}}/Fz_\alpha \cdot \mathcal{J}. \tag{S-11}$$

In the electroneutral case the electric current is given by $\mathcal{J} = \kappa \boldsymbol{E}$ in both frames.

## S-2 Experimental Validation

### S-2.1 Binary Systems

Table S1 contains the conductivities for all pure ionic liquid (IL) systems measured with impedance spectroscopy as well as the partial molar volumes of each ion calculated from density measurements. Conductivities are afflicted with a 10% error and partial molar volumes with 3%. For more details on the experimental specifics we refer to Ref. S3.

### S-2.2 Ternary Systems

Table S2 shows a list of the ternary mixtures and their composition used as database in section IV D.

**Table S1: List of ionic liquids (ILs) with their conductivity and ion partial molar volumes.**

| IL | conductivity $\kappa$ S/m | cation molar volume $\nu_+$ $10^{-6}$ $m^3$/mol | anion molar volume $\nu_-$ $10^{-6}$ $m^3$/mol |
|---|---|---|---|
| EMIM BF4 | 1.30 | 110.89 | 43.70 |
| EMIM TFSI | 0.80 | 107.13 | 147.26 |
| BMIM TFSI | 0.35 | 145.08 | 146.25 |
| Pyr14 TFSI | 0.23 | 156.32 | 145.91 |
| BMA TFSI | 0.15 | 139.71 | 144.38 |
| BmPip TFSI | 0.09 | 166.46 | 148.81 |
| BMIM PF6 | 0.12 | 144.21 | 63.10 |
| EMIM FSI | 1.52 | 114.84 | 87.42 |
| Pyr12O1 FSI | 0.63 | 144.61 | 91.06 |

**Table S2: List of ternary mixtures and their composition.**

| Parameter | Value | Source |
|---|---|---|
| EMIM BF4 1 | EMIM BF4 (0.962) Li BF4 (0.038) | Gouverneur 2018 [S4] |
| EMIM BF4 2 | EMIM BF4 (0.927) Li BF4 (0.073) | Gouverneur 2018 [S4] |
| EMIM BF4 3 | EMIM BF4 (0.86) Li BF4 (0.14) | this work |
| EMIM TFSI 1 | EMIM TFSI (0.938) Li TFSI (0.062) | Gouverneur 2018 [S4] |
| EMIM TFSI 2 | EMIM TFSI (0.879) Li TFSI (0.121) | Gouverneur 2018 [S4] |
| EMIM TFSI 3 | EMIM TFSI (0.9) Li TFSI (0.1) | this work |
| EMIM TFSI 4 | EMIM TFSI (0.86) Li TFSI (0.14) | this work |
| EMIM TFSI 5 | EMIM TFSI (0.7) Li TFSI (0.3) | this work |
| EMIM FSI 1 | EMIM FSI (0.9) Li FSI (0.1) | this work |
| EMIM FSI 2 | EMIM FSI (0.86) Li FSI (0.14) | this work |
| EMIM FSI 3 | EMIM FSI (0.7) Li FSI (0.3) | this work |
| Pyr12O1 TFSI | Pyr12O1 TFSI (0.6) Li TFSI (0.4) | this work |
| Pyr12O1 FSI | Pyr12O1 FSI (0.6) Li FSI (0.4) | this work |
| Pyr12O1 FTFSI 1 | Pyr12O1 FTFSI (0.9) Li FTFSI (0.1) | Brinkkötter 2021 [S5] |
| Pyr12O1 FTFSI 2 | Pyr12O1 FTFSI (0.8) Li FTFSI (0.2) | Brinkkötter 2021 [S5] |
| Pyr12O1 FTFSI 3 | Pyr12O1 FTFSI (0.7) Li FTFSI (0.3) | Brinkkötter 2021 [S5] |
| Pyr12O1 FTFSI 4 | Pyr12O1 FTFSI (0.6) Li FTFSI (0.4) | Brinkkötter 2021 [S5] |
| Pyr14 TFSI 1 | Pyr14 TFSI (0.9) Li TFSI (0.1) | this work |
| Pyr14 TFSI 2 | Pyr14 TFSI (0.86) Li TFSI (0.14) | this work |
| Pyr14 FSI 1 | Pyr14 FSI (0.9) Li FSI (0.1) | this work |
| Pyr14 FSI 2 | Pyr14 FSI (0.86) Li FSI (0.14) | this work |

The partial molar volumes of the ions are the same as in table S1 since they are assumed to be concentration-independent. For $Li^+$ the ionic radius of lithium (76 pm) was taken to calculate the volume in spherical approximation as $\nu_{Li^+0} = 1.11 \cdot 10^{-6}$ $m^3$/mol. Table S3 lists the ionic

conductivities measured by impedance spectroscopy as well as the transference numbers calculated from eq. (46).

**Table S3: List of conductivities and volume-based transference numbers for the ternary systems calculated from eq. (46).**

| System | Conductivity $\kappa$ in S/m | Transference numbers lithium $t^v_{Li^+}$ | cation $t^v_+$ | anion $t^v_-$ |
|---|---|---|---|---|
| EMIM BF4 1 | 1.230 ± 0.123 | −0.019 ± 0.004 | 0.526 ± 0.115 | 0.486 ± 0.101 |
| EMIM BF4 2 | 1.080 ± 0.108 | −0.039 ± 0.007 | 0.538 ± 0.127 | 0.459 ± 0.091 |
| EMIM BF4 3 | 0.756 ± 0.038 | −0.090 ± 0.021 | 0.438 ± 0.218 | 0.614 ± 0.188 |
| EMIM TFSI 1 | 0.653 ± 0.065 | −0.025 ± 0.007 | 0.485 ± 0.119 | 0.462 ± 0.108 |
| EMIM TFSI 2 | 0.542 ± 0.054 | −0.035 ± 0.005 | 0.592 ± 0.097 | 0.321 ± 0.107 |
| EMIM TFSI 3 | 0.550 ± 0.028 | −0.035 ± 0.015 | 0.790 ± 0.140 | 0.342 ± 0.078 |
| EMIM TFSI 4 | 0.450 ± 0.023 | −0.073 ± 0.014 | 0.576 ± 0.107 | 0.398 ± 0.160 |
| EMIM TFSI 5 | 0.171 ± 0.005 | −0.127 ± 0.026 | 0.732 ± 0.108 | 0.527 ± 0.080 |
| EMIM FSI 1 | 1.189 ± 0.060 | −0.022 ± 0.007 | 0.653 ± 0.074 | 0.496 ± 0.096 |
| EMIM FSI 2 | 1.061 ± 0.053 | −0.024 ± 0.010 | 0.548 ± 0.039 | 0.606 ± 0.175 |
| EMIM FSI 3 | 0.715 ± 0.022 | −0.081 ± 0.046 | 0.386 ± 0.140 | 0.670 ± 0.221 |
| Pyr12O1 TFSI | 0.024 ± 0.001 | −0.143 ± 0.034 | 0.544 ± 0.108 | 0.563 ± 0.139 |
| Pyr12O1 FSI | 0.192 ± 0.004 | 0.034 ± 0.015 | 0.328 ± 0.064 | 0.570 ± 0.078 |
| Pyr12O1 FTFSI 1 | 0.450 ± 0.009 | −0.025 ± 0.004 | 0.343 ± 0.041 | 0.478 ± 0.057 |
| Pyr12O1 FTFSI 2 | 0.251 ± 0.005 | −0.063 ± 0.011 | 0.361 ± 0.043 | 0.539 ± 0.065 |
| Pyr12O1 FTFSI 3 | 0.128 ± 0.003 | −0.091 ± 0.015 | 0.494 ± 0.059 | 0.618 ± 0.074 |
| Pyr12O1 FTFSI 4 | 0.068 ± 0.001 | −0.098 ± 0.017 | 0.462 ± 0.055 | 0.604 ± 0.072 |
| Pyr14 TFSI 1 | 0.146 ± 0.007 | −0.040 ± 0.008 | 0.538 ± 0.041 | 0.615 ± 0.137 |
| Pyr14 TFSI 2 | 0.114 ± 0.006 | −0.053 ± 0.012 | 0.520 ± 0.042 | 0.608 ± 0.082 |
| Pyr14 FSI 1 | 0.343 ± 0.031 | −0.047 ± 0.010 | 0.506 ± 0.144 | 0.800 ± 0.277 |
| Pyr14 FSI 2 | 0.337 ± 0.038 | −0.052 ± 0.022 | 0.471 ± 0.121 | 0.909 ± 0.246 |

# References


(S1) Schammer, M.; Horstmann, B.; Latz, A. Theory of Transport in Highly Concentrated Electrolytes. *Journal of the Electrochemical Society* **2021**, *168*, 026511.

(S2) Goyal, P.; Monroe, C. W. New Foundations of Newman's Theory for Solid Electrolytes: Thermodynamics and Transient Balances. *Journal of The Electrochemical Society* **2017**, *164*, E3647–E3660.

(S3) Lorenz, M.; Kilchert, F.; Nürnberg, P.; Schammer, M.; Latz, A.; Horstmann, B.; Schönhoff, M. Local volume conservation in concentrated electrolytes is governing charge transport in electric fields. 2022.

(S4) Gouverneur, M.; Schmidt, F.; Schönhoff, M. Negative effective Li transference numbers in Li salt/ionic liquid mixtures: Does Li drift in the "wrong" direction? *Physical Chemistry Chemical Physics* **2018**, *20*, 7470–7478.

(S5) Brinkkötter, M.; Mariani, A.; Jeong, S.; Passerini, S.; Schönhoff, M. Ionic Liquid in Li Salt Electrolyte: Modifying the Li+ Transport Mechanism by Coordination to an Asymmetric Anion. *Advanced Energy and Sustainability Research* **2021**, *2*, 2000078.
